# Supplementary material for: Using Transfer Learning for Image-Based Cassava Disease Detection
Source: arXiv:1707.03717 source file (2017-08-01)
Supplement: Supplementary file 1 [file frontiers_SupplementaryMaterial.tex]

%%%%%%%%%%%%%%%%%%%%%%%%%%%%%%%%%%%%%%%%%%%%%%%%%%%%%%%%%%%%%%%%%%%%%%%%%%%%%%%%%%%%%%%%%%%%%%%%%%%%%%%%%%%%%%%%%%%%%%%%%%%%%%%%%%%%%%%%%%%%%%%%%%%%%%%%%%%
% This is just an example/guide for you to refer to when producing your supplementary material for your Frontiers article.                                 %
%%%%%%%%%%%%%%%%%%%%%%%%%%%%%%%%%%%%%%%%%%%%%%%%%%%%%%%%%%%%%%%%%%%%%%%%%%%%%%%%%%%%%%%%%%%%%%%%%%%%%%%%%%%%%%%%%%%%%%%%%%%%%%%%%%%%%%%%%%%%%%%%%%%%%%%%%%%

%%% Version 2.3 Generated 2016/11/10 %%%
%%% You will need to have the following packages installed: datetime, fmtcount, etoolbox, fcprefix, which are normally inlcuded in WinEdt. %%%
%%% In http://www.ctan.org/ you can find the packages and how to install them, if necessary. %%%
%%%  NB 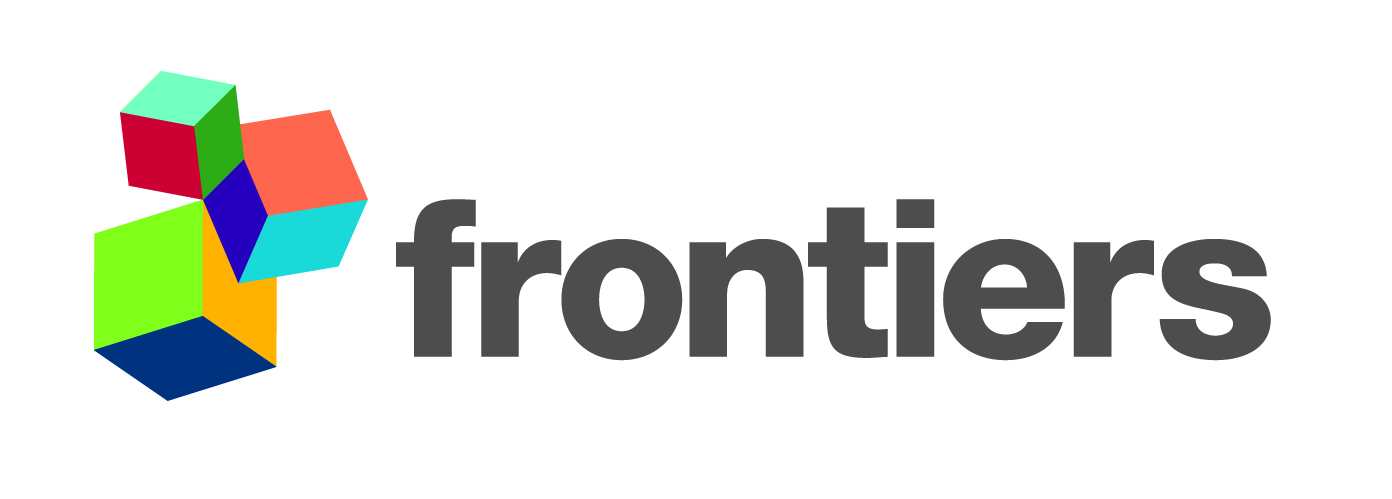 is required in the path in order to correctly compile front page header %%%

\documentclass[utf8]{frontiers_suppmat} % for all articles
\usepackage{url,hyperref,lineno,microtype,subcaption}
\usepackage[onehalfspacing]{setspace}

% Leave a blank line between paragraphs in stead of using \\

\def\firstAuthorLast{Frontiers} 
\def\Authors{First Author, Co-Author* and Co-Author}
% The Corresponding Author should be marked with an asterisk
% Provide email of the corresponding author

\begin{document}
\onecolumn
\firstpage{1}

\title[Supplementary Material]{{\helveticaitalic{Supplementary Material}}:
\\ \helvetica{Article Title}} %Please insert the title of your article here

\author[\firstAuthorLast ]{\Authors} %This field will be automatically populated
\correspondance{} %This field will be automatically populated

\extraAuth{}% If there are more than 1 corresponding author, comment this line and uncomment the next one.
%\extraAuth{Corresponding Author2: email2@uni2.edu}

\maketitle

\section{Supplementary Data}

Supplementary Material should be uploaded separately on submission. Please include any supplementary data, figures and/or tables. 

Supplementary material is not typeset so please ensure that all information is clearly presented, the appropriate caption is included in the file and not in the manuscript, and that the style conforms to the rest of the article. 

\section{Supplementary Tables and Figures}

For more information on Supplementary Material and for details on the different file types accepted, please see  \href{http://home.frontiersin.org/about/author-guidelines#SupplementaryMaterial}{the Supplementary Material section}  of the Author Guidelines.

\subsection{Figures}

%%% There is no need for adding the file termination, as long as you indicate where the file is saved. In the examples below the files (logo1.jpg and 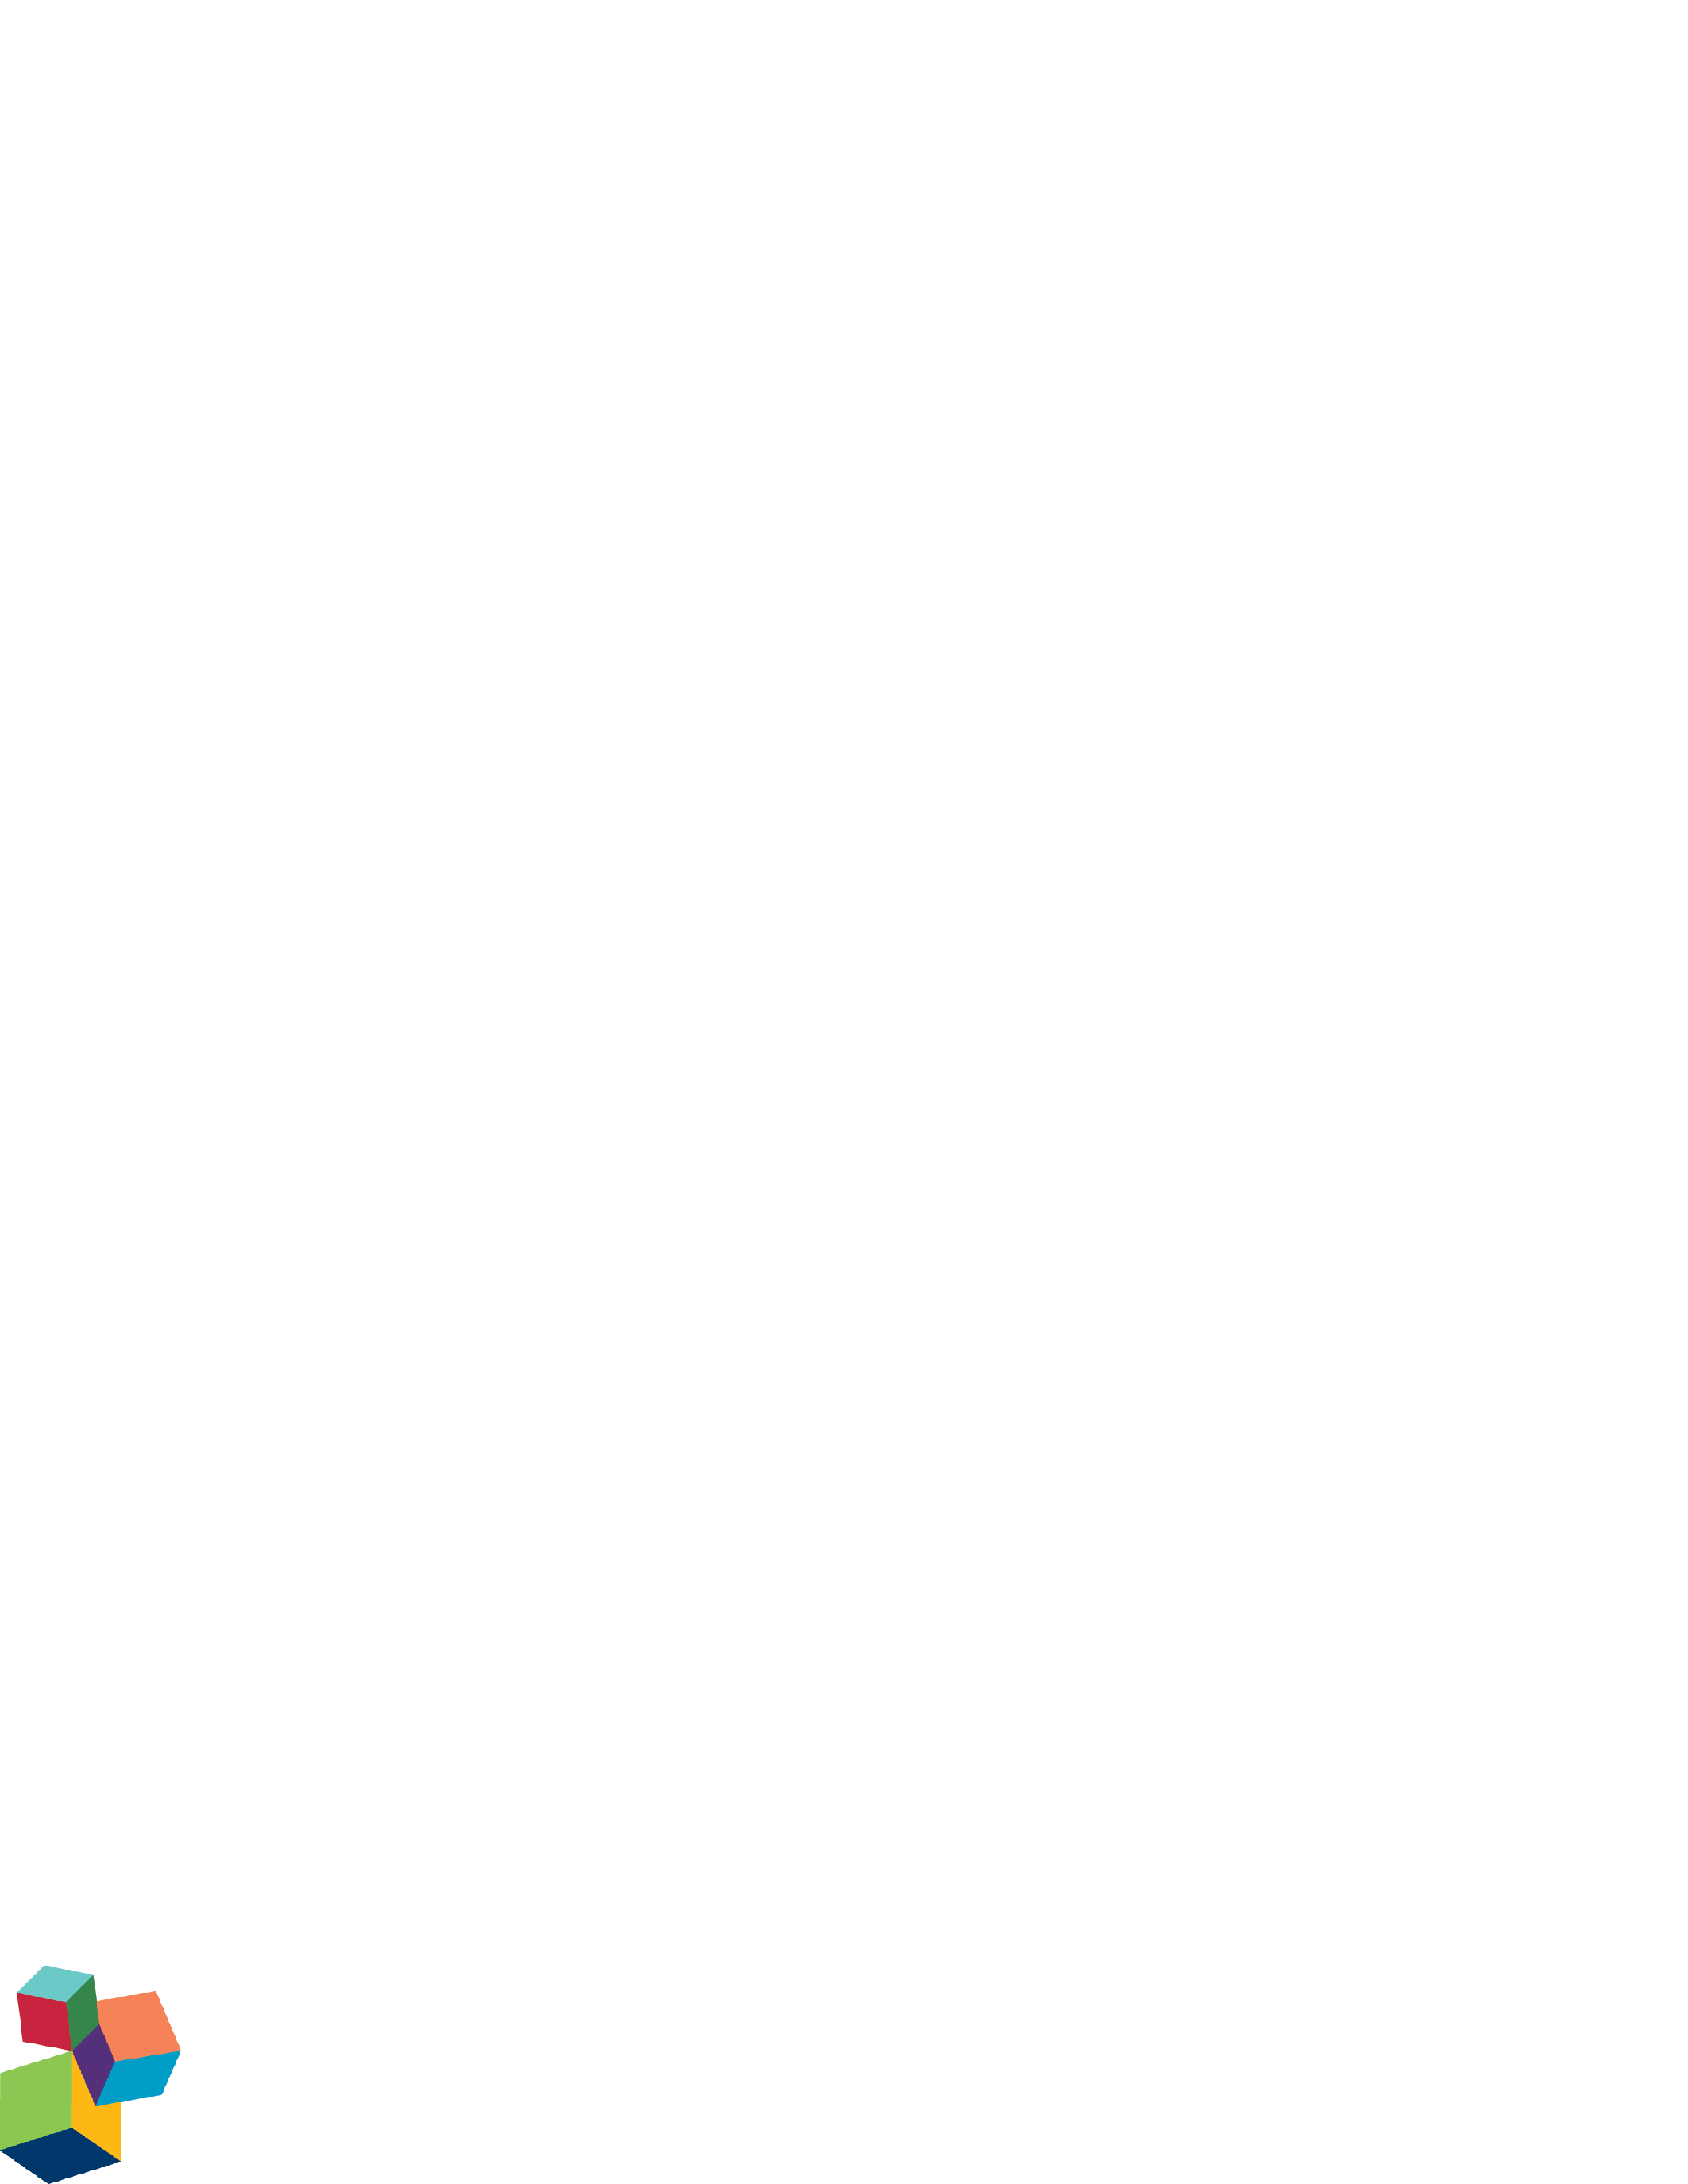) are in the Frontiers LaTeX folder
%%% If using *.tif files convert them to .jpg or .png
%%% If using panelled/compiled figures with subcaptions, use the subcaption package as in the second example.  N.B. This package is incompatible with the subfigure and subfig packages
%%%  NB logo1.jpg is required in the path in order to correctly compile front page header %%%

\begin{figure}[h!]
\begin{center}
\includegraphics[width=10cm]{logo1}% This is a *.jpg file
\end{center}
\caption{ Enter the caption for your figure here.  Repeat as  necessary for each of your figures}\label{fig:1}
\end{figure}

\begin{figure}[h!]
\begin{minipage}[b]{.5\linewidth}
\centering\includegraphics[width=6cm]{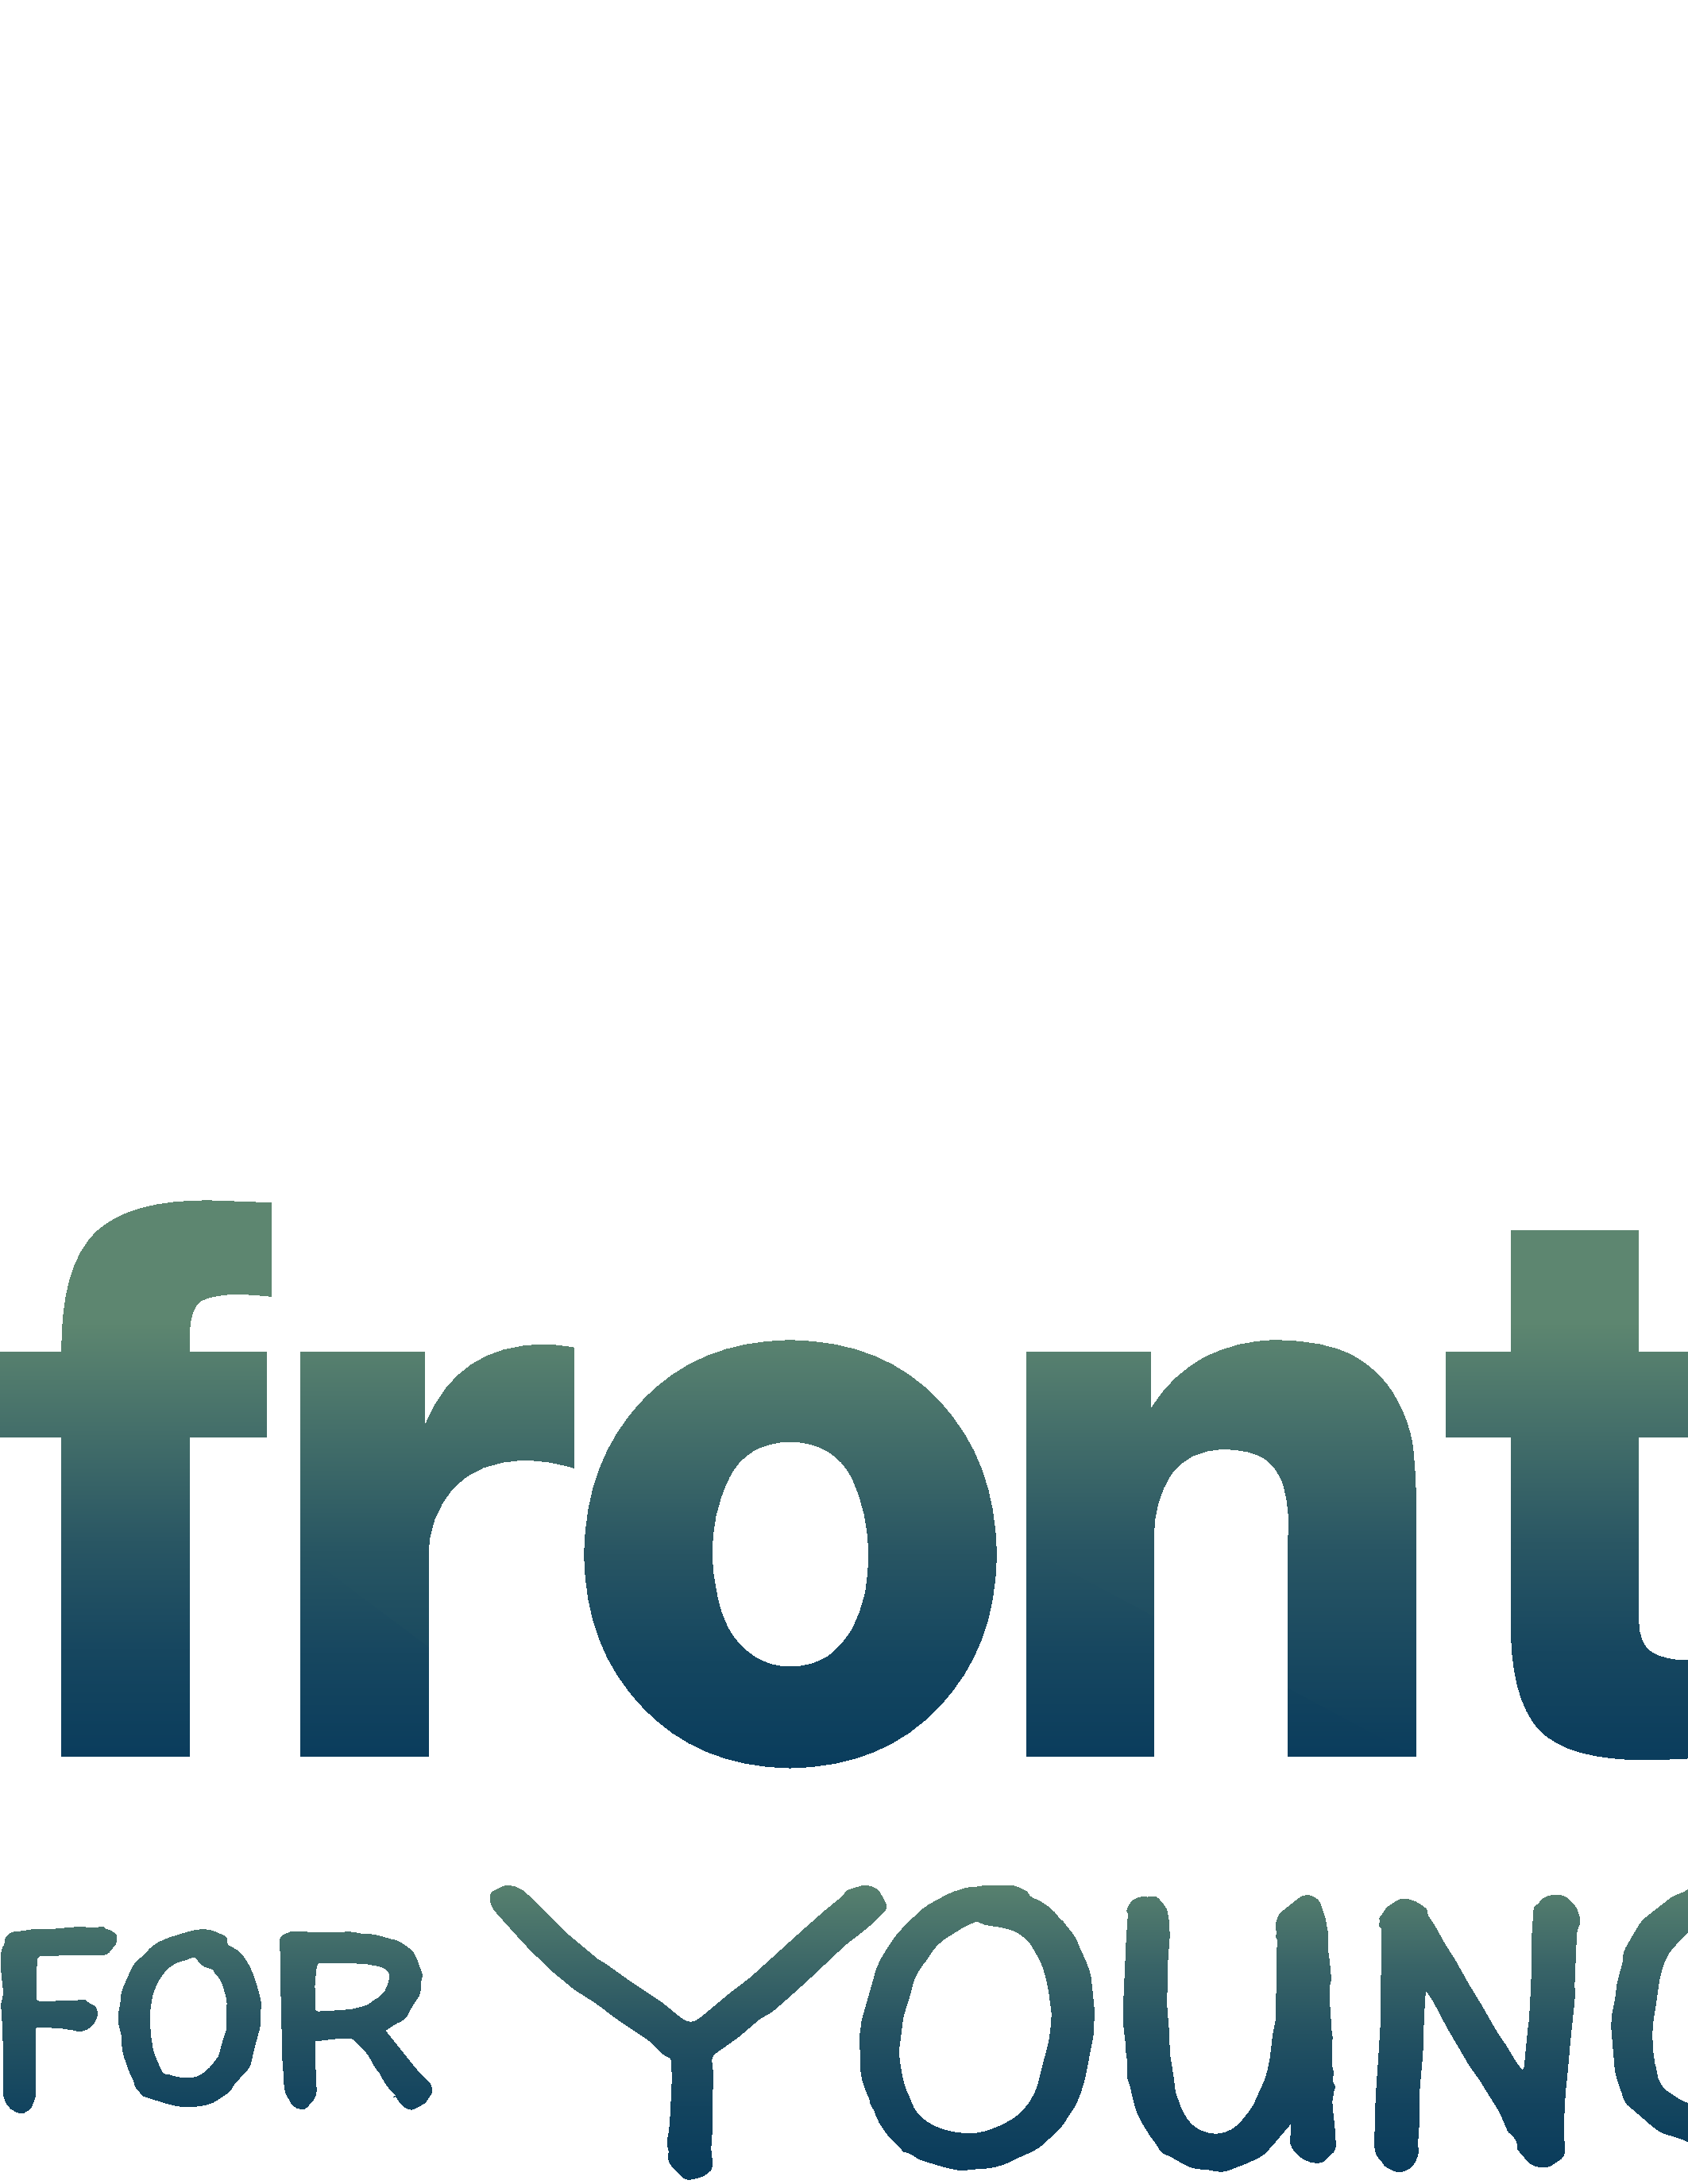}% This is a *.eps file
\subcaption{A subfigure}\label{fig:2a}
\end{minipage}%
\begin{minipage}[b]{.5\linewidth}
\centering\includegraphics[width=2cm]{logo2}% This is an *.eps file
\subcaption{Another subfigure}\label{fig:2b}
\end{minipage}
\caption{A figure}\label{fig:2b}
\end{figure}

%\bibliographystyle{frontiersinSCNS_ENG_HUMS} %  for Science, Engineering and Humanities and Social Sciences articles, for Humanities and Social Sciences articles please include page numbers in the in-text citations
%\bibliographystyle{frontiersinHLTH&FPHY} % for Health and Physics articles
%\bibliography{test}

\end{document}
